# Supplementary material for: Discovering Nested Communities
Source: arXiv:1902.01483 source file (2019-02-04)
Supplement: Supplementary file 1 [file appendix.tex]

\appendix
\section{Proofs}
\label{sec:apx}

\begin{proof}[of Proposition~\ref{prop:gain}]
Let $i = \tid{X; \tree{T}}$. It follows directly from the definition that for
any tile $Z \in \tree{T}$ we have $\tid{Z; \tree{T}'} = \tid{Z; \tree{T}}$ if $\tid{Z;
\tree{T}} < i$, while $\tid{Z; \tree{T}'} = \tid{Z; \tree{T}} + 1$ if $\tid{Z;
\tree{T}} \geq i$. We also have $i = \tid{Y; \tree{T}'}$. This implies that $\cells{Q; \tree{T}} = \cells{Q; \tree{T}'}$ for any $Q \in \tree{T}$
such that $Q \neq X$, which implies that $\lc{D \mid Q, \tree{T}} = \lc{D \mid Q, \tree{T}'}$.
Consequently, we have
\[
\begin{split}
	\lc{D, \tree{T}'} - \lc{D, \tree{T}} & = \lc{D \mid Y, \tree{T}'} + \lc{D \mid X, \tree{T}'} - \lc{D \mid X, \tree{T}} +  \lc{Y \mid \tree{T}'} \\
	& = \ent{u, v} + \lc{D \mid X, \tree{T}'} - \ent{o, z} + \lc{Y \mid \tree{T}'}\quad.
\end{split}
\]
Since $\cells{Y; \tree{T}'} \subseteq \cells{X; \tree{T}}$,
we have $\ones{X; \tree{T}'} = o - u$ and $\zeroes{X; \tree{T}'} = z - v$.
\qed\end{proof}

\begin{lemma}
\label{lem:inequality}
Define $g(x, y, o, z) = \ent{x, y} + \ent{o - x, z - y}$.
Assume $8$ non-negative numbers $r_p$, $r_n$, $s_p$, $s_n$, $t_p$, $t_n$, $o$, $z$. 
Assume that $t_p + t_n > 0$ and $s_p + s_n > 0$ and $t_p / (t_p + t_n) \geq s_p / (s_p + s_n)$.
Write $u = r_p + s_p$ and $v = r_n + s_n$.
Assume that $u + t_p \leq o$, $v + t_n \leq z$, and $u / (u + v) > o / (o + z)$.
Let $q = g(u, v, o, z)$. Then either $g(r_p, r_n, o, z) < q$ or $g(u + t_p, v + t_n, o, z) \leq q$.
\end{lemma}

\begin{proof}
Assume that $g(r_p, r_n, o, z) \geq q$.
Note that because of $u / (u + v) > o / (o + z)$ we must have $u > 0$ and $v < z$.
Assume that $0 < v$ and $u < o$.
Define 
\[
\begin{split}
	A = -\log \frac{u}{u + v}&,\ 
	B = -\log \frac{v}{u + v},\  \\
	C = -\log \frac{o - u}{o + z - u + v}&,\ 
	D = -\log \frac{z - v}{o + z - u + v}\quad.
\end{split}
\]
Define $h(x, y) = xA + yB + (o - x)C + (z - y)D$.
Since $h(x, y)$ is essentially the length of encoding with possibly sub-optimal codes, it follows that
\begin{equation}
\label{eq:bound}
	g(x, y, o, z) \leq h(x, y) \text{ and } g(u, v, o, z) = h(u, v)\quad.
\end{equation}

Define $f(x, n) = n(x(A - C) + (1 - x)(B - D))$.
We have the following identity between $h$ and $f$,
\[
\begin{split}
	h(x, y) - h(u, v) & = (x - u)(A - C) + (y - v)(B - D) \\
	& = f( (x - u) /(x + y - u - v) , x + y - u - v)\quad.
\end{split}
\]
Since $u / (u + v) > o / (o + z)$, we have $A < C$ and $D < B$,
which implies that $f(x, n)$ is non-increasing w.r.t to $x$ for any $n \geq 0$.

Let $m = s_p + s_n$ and define $w = s_p / m$. We have
\[
	0 \geq g(u, v, o, z) - g(r_p, r_n, o, z) \geq h(u, v) - h(r_p, r_n) = -f(w, -m) = f(w, m)\quad.
\]

This implies that $f(w, n) \leq 0$ for any $n \geq 0$. Since $t_p / (t_p + t_n) \geq w$,
we have $f(t_p / (t_p + t_n), t_p + t_n) \leq 0$. This implies that
\[
\begin{split}
	g(u + t_p, v + t_n, o, z) - g(u, v, o, z) & \leq h(u + t_p, v + t_n) - h(u, v) \\
	& = f(t_p / (t_p + t_n), t_p + t_n) \leq 0\quad.
\end{split}
\]

Assume now that $v = 0$, this will make $B = \infty$. However, we can repeat
the proof as long as $D < B$ and Eq.~\ref{eq:bound} is satisfied. This can be
done if we select $B$ high enough, say $B = \max g(x, y, o, z)$, where $0 \leq
x \leq o$ and $0 \leq y \leq z$. The argument is similar for case $u = o$.
\qed\end{proof}

\begin{proof}[of Proposition~\ref{prop:inequality}]
We will only show the case that there exist $a$ and $b$ such that $\cost{u, v} \leq \cost{i, j}$
and $a$ is a head border of $b$. The proofs for other cases are similar.

Assume that $i$ is not a head border of $j$. There exist
indices $1 \leq x < i \leq y \leq j$ such that $\freq{x, i - 1} \geq \freq{i, y}$.
Let
$r_p = \cnt{y + 1, j; p}$,
$r_n = \cnt{y + 1, j; n}$,
$s_p = \cnt{i, y ; p}$,
$s_n = \cnt{i, y ; n}$,
$t_p = \cnt{x, i - 1 ; p}$,
$t_n = \cnt{x, i - 1 ; n}$.
Then the conditions in Lemma~\ref{lem:inequality} are satisfied. Hence either
$\cost{y + 1, j} < \cost{i, j}$ or $\cost{x, j} \leq \cost{i, j}$.
Note that in the first case we must have $y + 1 \leq j$ since $\cost{i, j} \leq \cost{j + 1, j} = \ent{o, z}$.
We can now reset $a = y + 1$ or to $a = x$ if it is the second case, and repeat the argument.
Note that during each step we either decrease the score or move $i$ to the left. Since there
are only finite number of possible scores, this process will eventually stop and we have found
$a = i$ that is a head border of $b = j$.
\qed\end{proof}
